# Supplementary material for: Printing on particles: combining two-photon nanolithography and capillary assembly to fabricate multi-material microstructures
Source: arXiv:2208.02635 source file (2022-08-04)
Supplement: Supplementary file 2 [file printing_code.tex]

\documentclass{article}
\usepackage{minted}
\begin{document}
\newminted{python}{
    fontsize=\footnotesize, 
    escapeinside=||,
    mathescape=true,
    numbersep=5pt,
    linenos=true,
    autogobble,
    framesep=3mm}

\inputminted{python}{printingOnParticles.py}

\end{document}
